# Supplementary material for: Multispectral Demosaicing via Dual Cameras
Source: arXiv:2503.22026 source file (2025-07-25)
Supplement: Supplementary file 1 [file scene_pos_supp.pdf]

Image samples of scenes captured in various camera positions

Scenes staged in the illumination box

#03

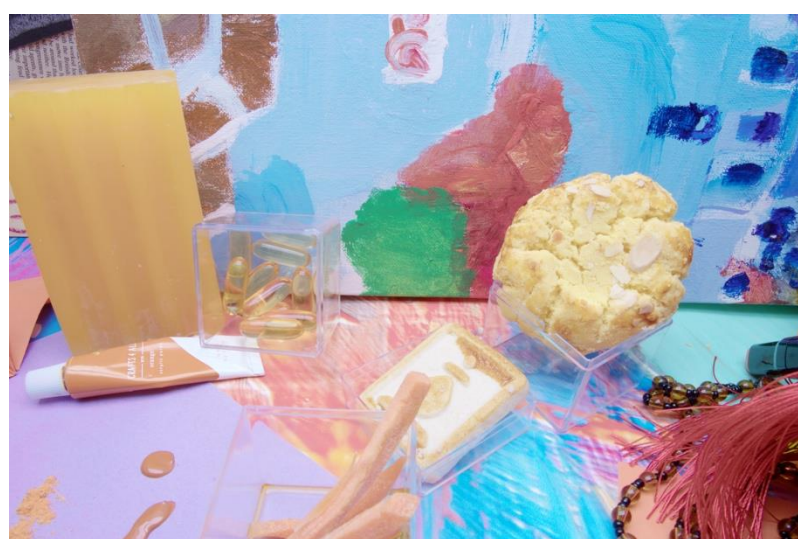

.....

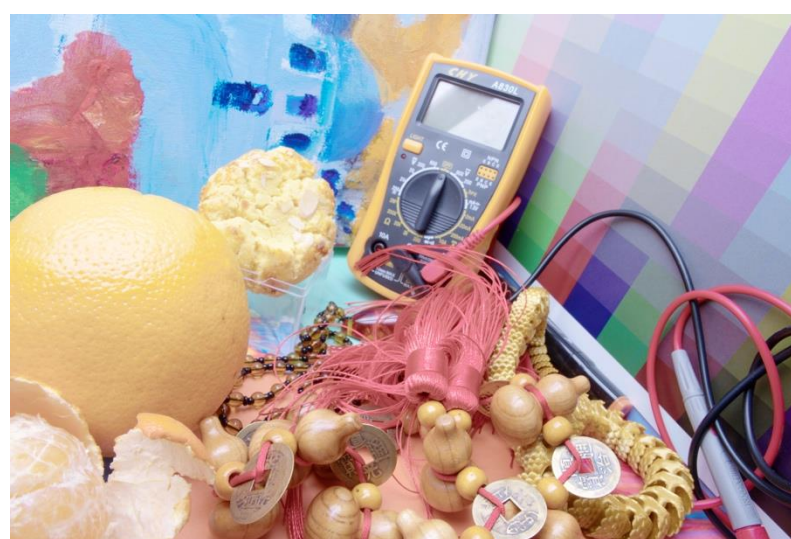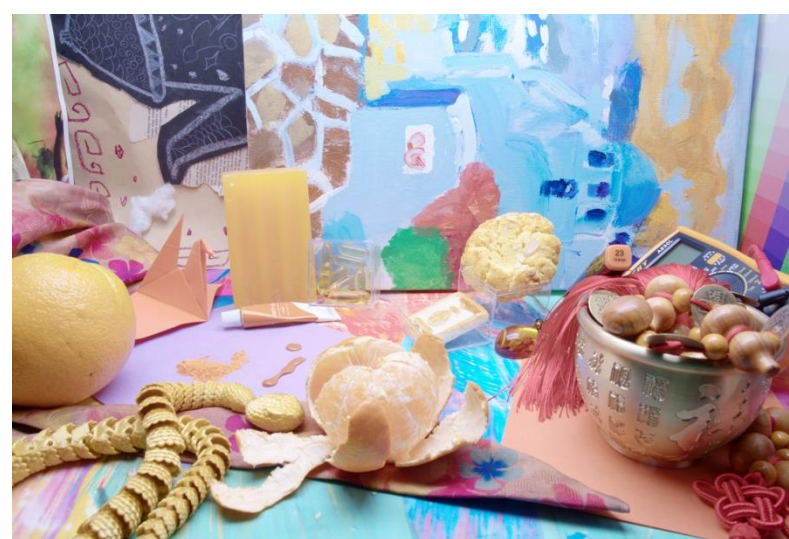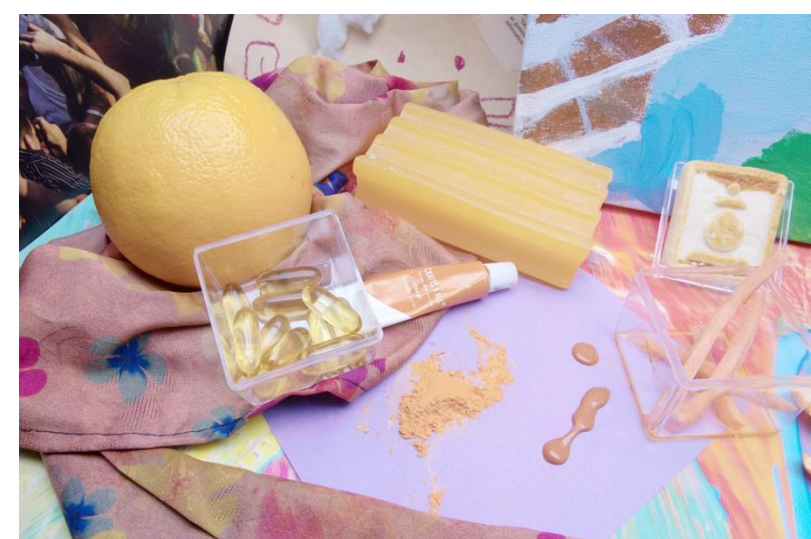

#10

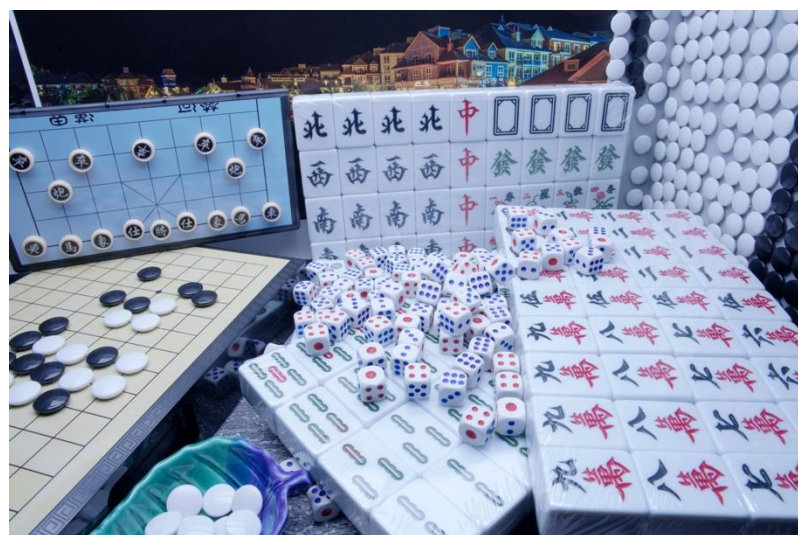

.....

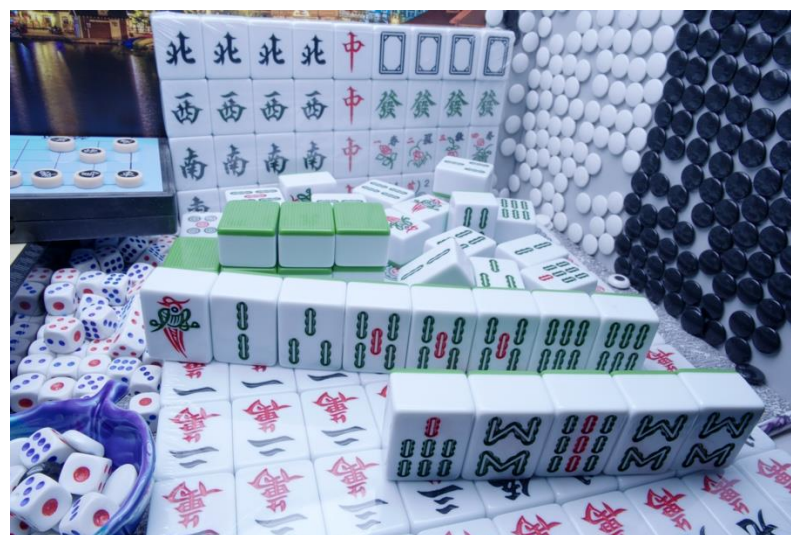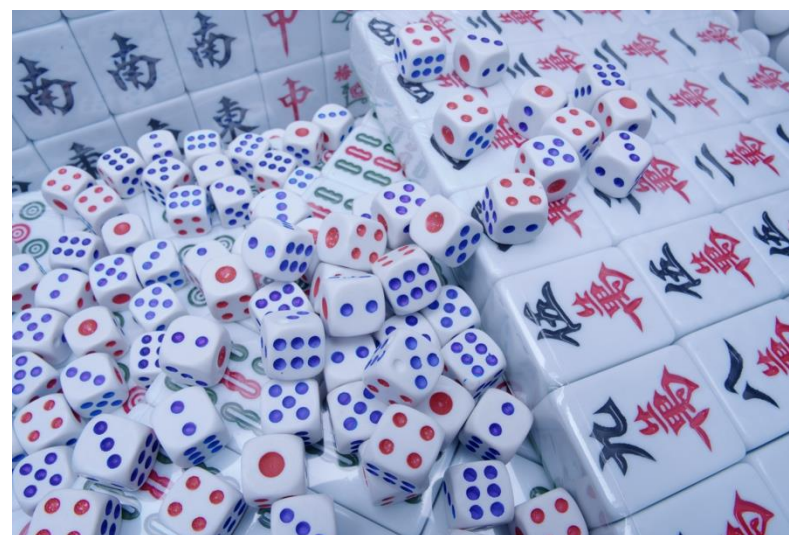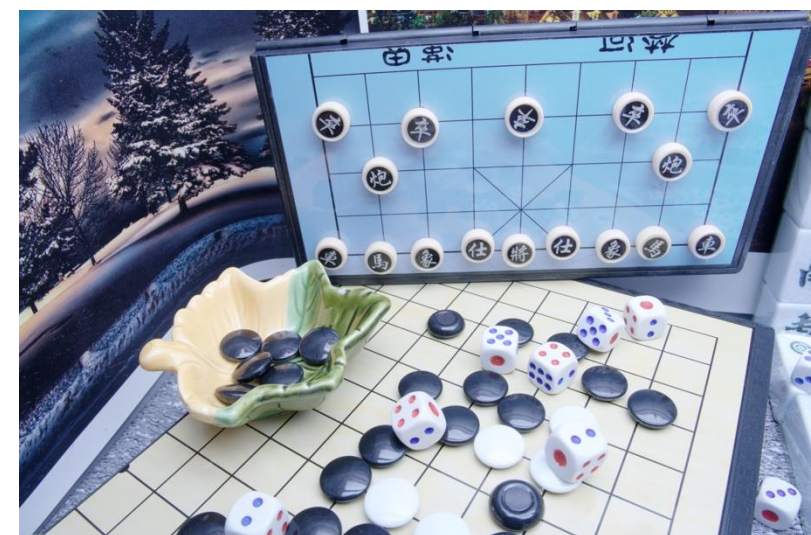

#13

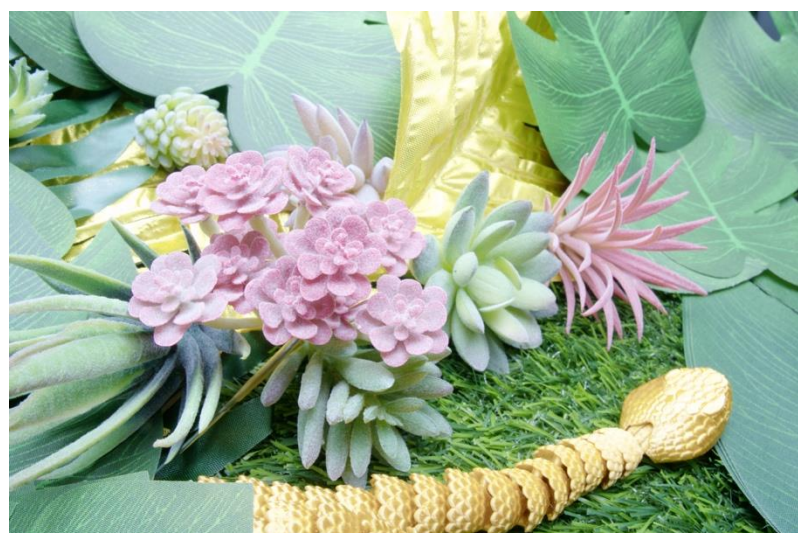

.....

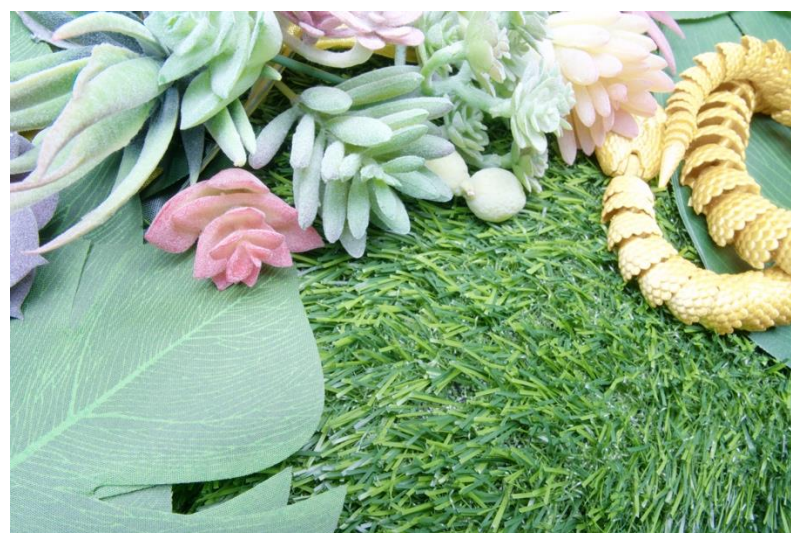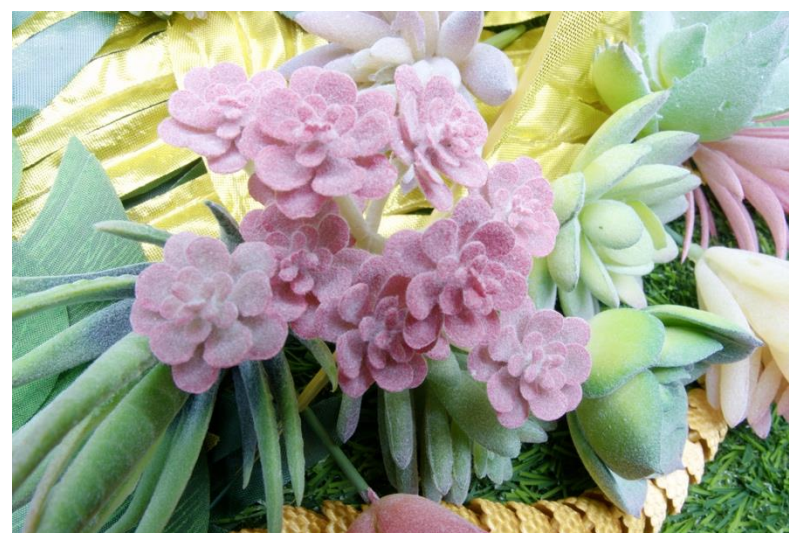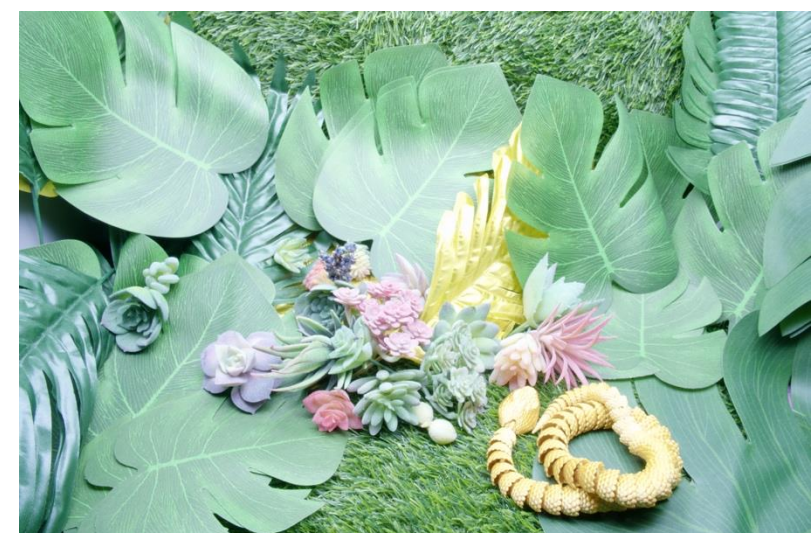

#16

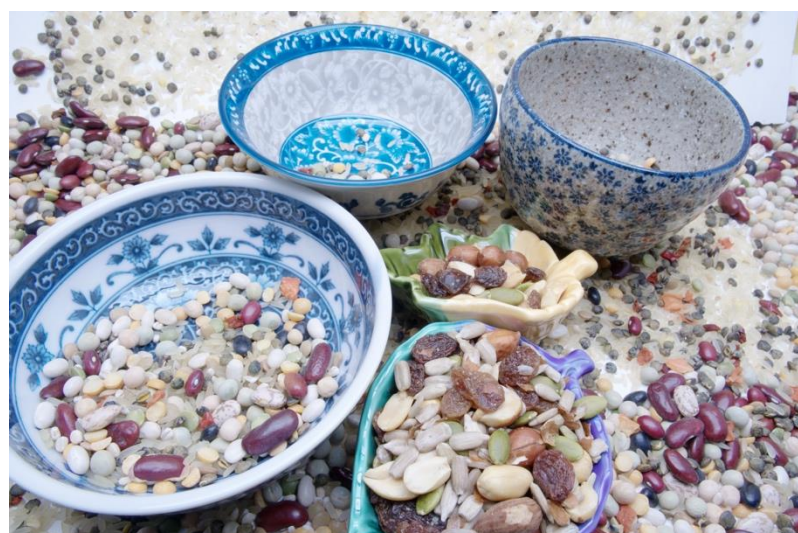

.....

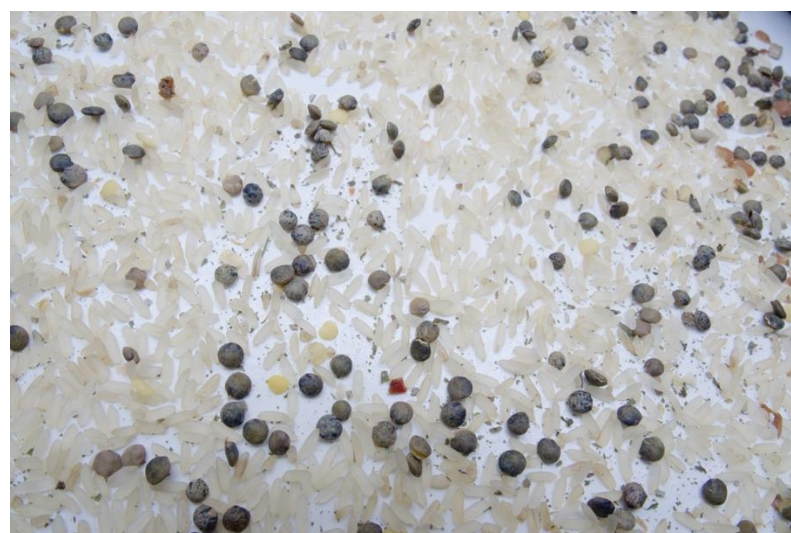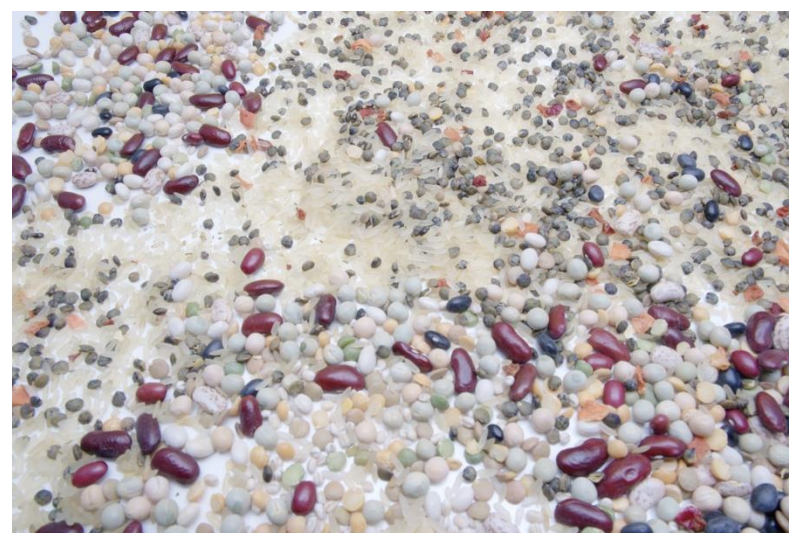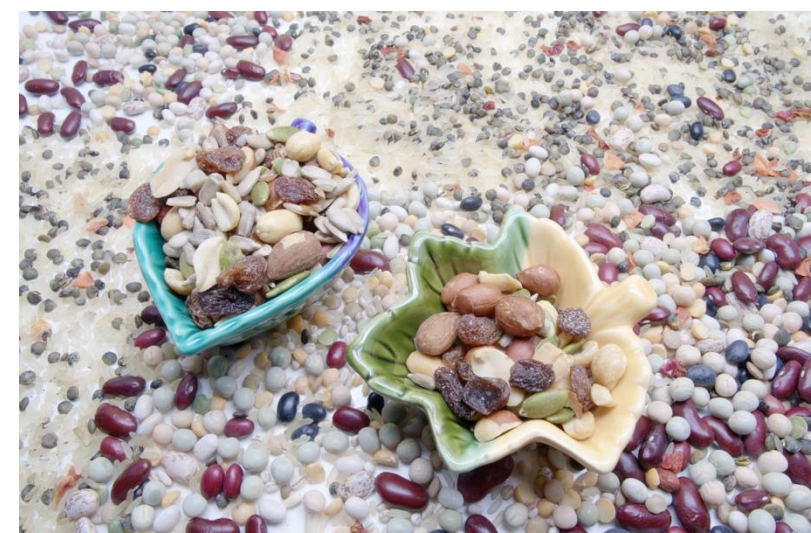

#26

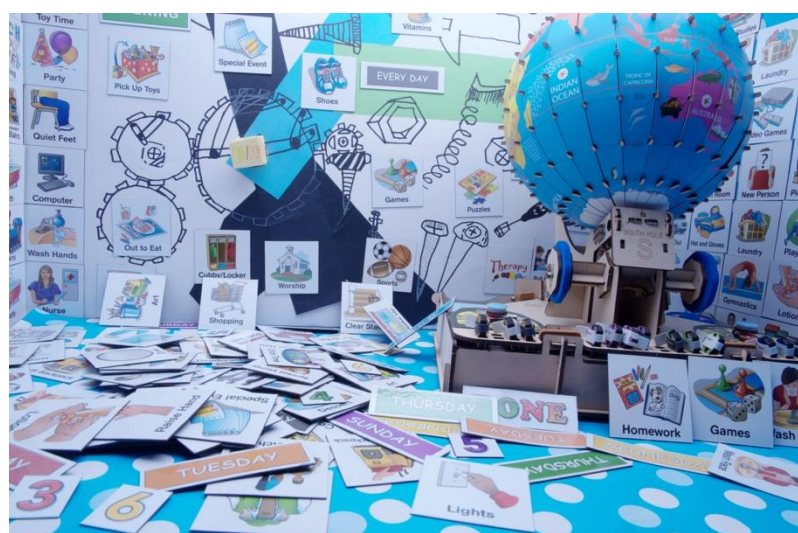

.....

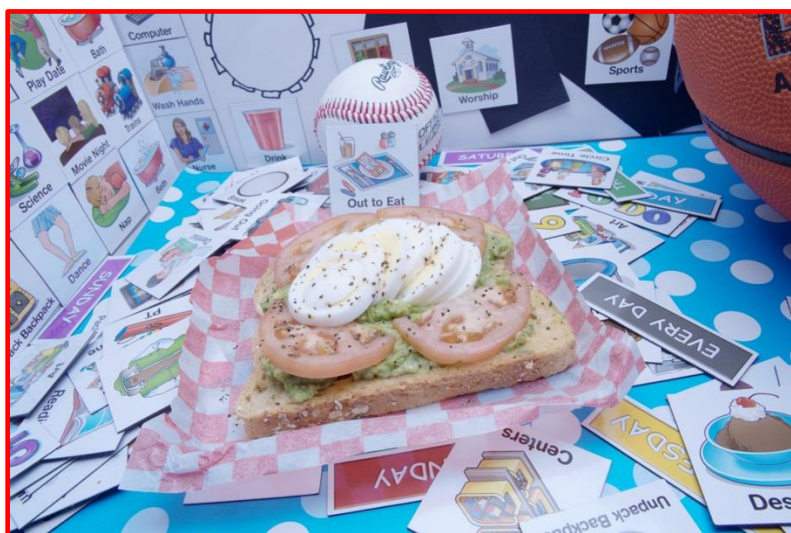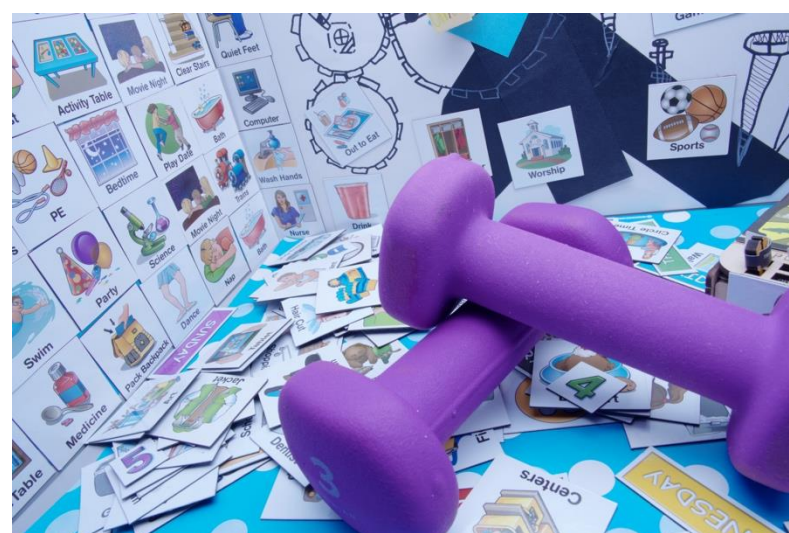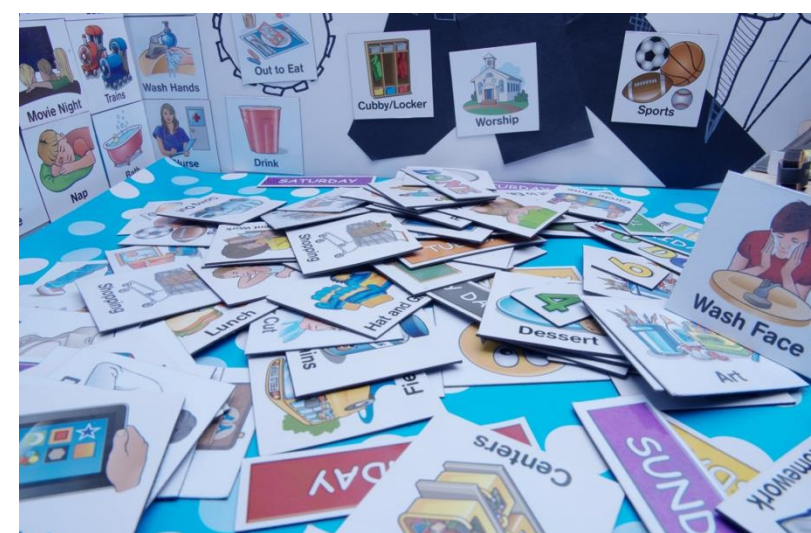

RGB CFA  
response  
function

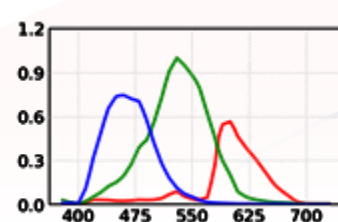

Dual-camera  
RGB-MS imaging system

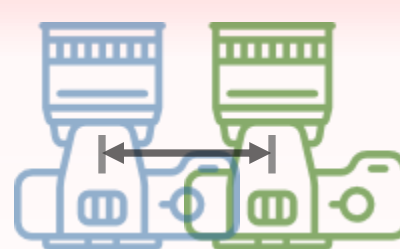

MSFA  
response  
function  
(simulated)

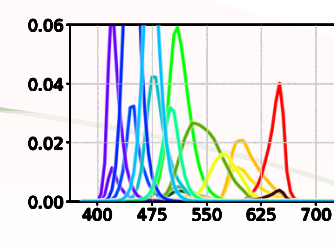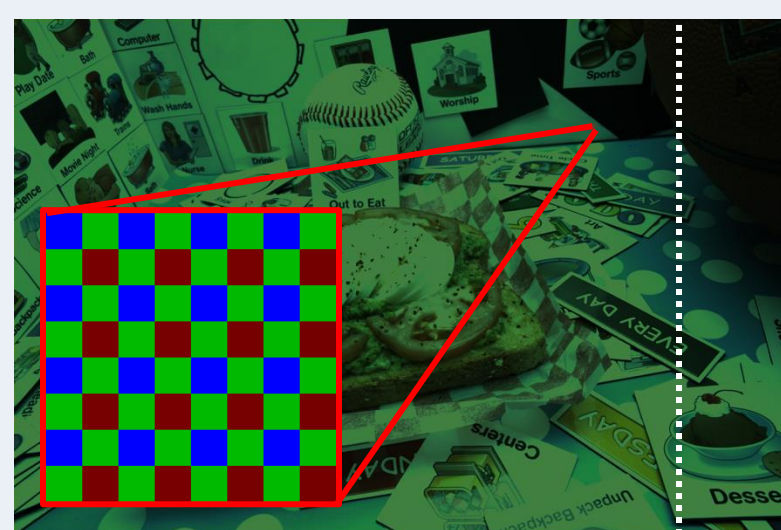

realistic  
RGB mosaic image  
( $I_{2 \times 2}^{RGB}$ )

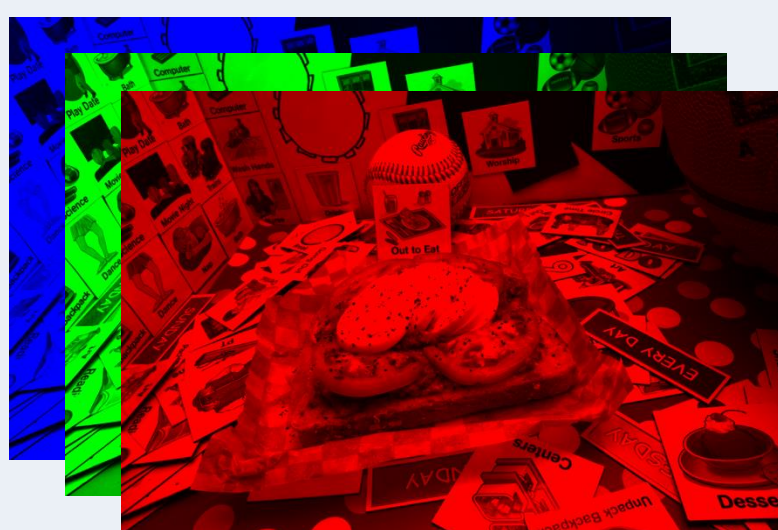

ground-truth  
RGB demosaic image  
( $\hat{I}^{RGB}$ )

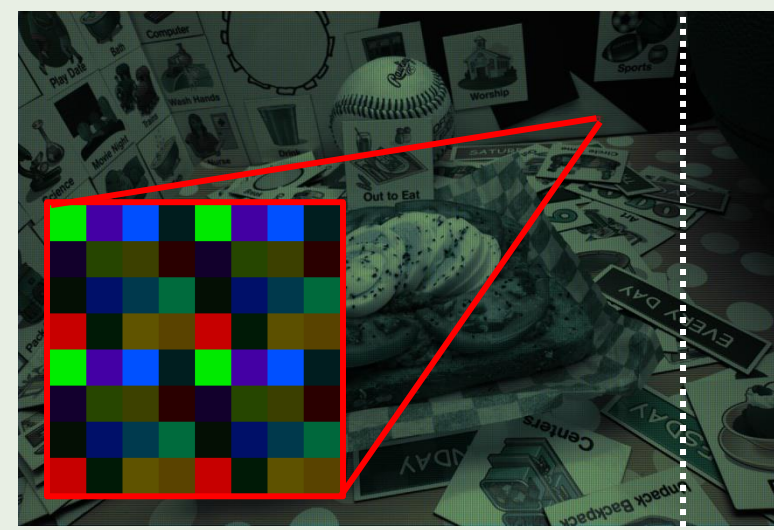

realistic  
MS mosaic image  
( $I_{4 \times 4}^{MS}$ )

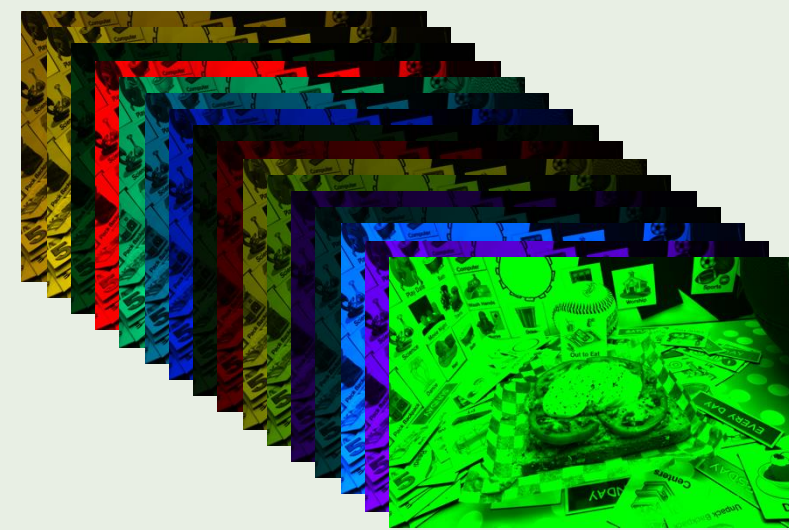

ground-truth  
MS demosaic image  
( $\hat{I}^{MS}$ )
